# Supplementary material for: GST-Bench: Can VLMs Develop Global Spatial Awareness from Video?
Source: arXiv:2608.05747 source file (2026-08-06)
Supplement: Supplementary file 1 [file appendix.tex]

\section{Experiment details}

\subsection{Fundamental Evaluation Prompts}
\label{appx:base}
The prompt templates for all benchmarks are listed below. In each template, \texttt{\{question\}} is replaced with the sample’s actual question, \texttt{\{options\}} with its multiple-choice answer options, \texttt{<image>} with the computed ViT embeddings of the input image, and \texttt{<video>} with the ViT embeddings of the video frames (for video benchmarks).

\paragraph{VSIBench.} We use the official metric of VSIBench~\cite{yang2025thinking}.

\begin{tcolorbox}
[colback=white,colframe=black,left=1mm,right=1mm,top=1mm,bottom=1mm]
\ttfamily
% \textbf{Appearance Order}

<video>

\texttt{\{question\}}

Options: \texttt{\{options\}}

Answer with the option's letter from the given choices directly.
\end{tcolorbox}

\paragraph{BLINK.} 
Following RoboBrain 2.0~\cite{team2025robobrain}, we evaluate BLINK~\cite{fu2024blink} on two sub-tasks—spatial relation understanding and depth perception—and report the average accuracy across them.

\begin{tcolorbox}
[colback=white,colframe=black,left=1mm,right=1mm,top=1mm,bottom=1mm]
\ttfamily
% \textbf{Appearance Order}

<image>

\texttt{\{question\}}

\texttt{\{options\}}

 Answer with the option's letter from the given choices directly.
\end{tcolorbox}

\paragraph{CV-Bench.} We follow the official evaluation protocol of CV-Bench~\cite{tong2024cambrian} and report average accuracy over the three defined sub-tasks.

\begin{tcolorbox}
[colback=white,colframe=black,left=1mm,right=1mm,top=1mm,bottom=1mm]
\ttfamily
% \textbf{Appearance Order}

<image>

\texttt{\{question\}}

\texttt{\{options\}}

 Answer with the option's letter from the given choices directly.
\end{tcolorbox}

\paragraph{EmbSpatial.} We use the official metric of EmbSpatial-Bench~\cite{du2024embspatial} and report the average accuracy.

\begin{tcolorbox}
[colback=white,colframe=black,left=1mm,right=1mm,top=1mm,bottom=1mm]
\ttfamily
% \textbf{Appearance Order}

<image>

\texttt{\{question\}}

 Please answer with a single option letter:
 
 \texttt{\{options\}}

\end{tcolorbox}

\paragraph{SAT.}  We use the official metric of SAT~\cite{ray2024sat} and report the average accuracy across its five sub-tasks.
% 4次api
\begin{tcolorbox}
[colback=white,colframe=black,left=1mm,right=1mm,top=1mm,bottom=1mm]
\ttfamily
% \textbf{Appearance Order}

<image>

\texttt{\{question\}}
 
 \texttt{\{options\}}

 Please only answer with the option letter.

\end{tcolorbox}

\paragraph{VSR.} We use the official metric of VSR~\cite{liu2023vsr} and report the average accuracy.

\begin{tcolorbox}
[colback=white,colframe=black,left=1mm,right=1mm,top=1mm,bottom=1mm]
\ttfamily
% \textbf{Appearance Order}

<image>

\texttt{\{question\}}

Answer with a single word yes or no.

\end{tcolorbox}

\paragraph{SpatialBench.} 
% Following RoboSpatial, we only report the accuracy of SpatialBench in terms of the position category.
We use the official metric of SpatialBench~\cite{du2024embspatial}.


\begin{tcolorbox}
[colback=white,colframe=black,left=1mm,right=1mm,top=1mm,bottom=1mm]
\ttfamily
% \textbf{Appearance Order}

<image>

\{question\}

Please answer with a single word: yes or no (for existence task).

\end{tcolorbox}


\paragraph{DA-2k.} Since some VLMs tend to repeatedly output the same option on DA-2k~\cite{yang2024depth}, we shuffle the answer choices and report the average accuracy.

\begin{tcolorbox}
[colback=white,colframe=black,left=1mm,right=1mm,top=1mm,bottom=1mm]
\ttfamily
% \textbf{Appearance Order}

<image>

\texttt{\{question\}}
 
Only provide the answer: point1 or point2.

\end{tcolorbox}

\paragraph{LVIS.} We report results on LVIS~\cite{gupta2019lvis} using the F1-score~\footnote{Since the baseline models (\eg{}, Qwen-2.5-VL, Cosmos-Reason1, RoboBrain-2.0, etc.) cannot follow a unified output format on the visual grounding benchmarks—including LVIS, RefCOCO, Pixmo-Point, and Where2Place—we revise their prompts to adapt to their output formats.}.
\begin{tcolorbox}
[colback=white,colframe=black,left=1mm,right=1mm,top=1mm,bottom=1mm]
\ttfamily
<image>

Ground all \texttt{\{object\}} in this image. Please provide all bounding box coordinates in the format: <|box\_start|>(x1, y1),(x2, y2)<|box\_end|>.

\vspace{1em}

Each bounding box should contain: 

- (x1, y1): the coordinates of the upper-left corner

- (x2, y2): the coordinates of the lower-right corner 

\vspace{1em}

All coordinates must be **normalized to the range [0, 1000]**, where:

- x refers to the horizontal axis (image width)

- y refers to the vertical axis (image height) 

\vspace{1em}

If **no object is detected**, simply output:  **No instance found.**
\end{tcolorbox}

\paragraph{RefCOCO \& RefCOCO+ \& RefCOCOg \& RefCOCOu.} We use the official metric of RefCOCO~\cite{yu2016modeling}.
\begin{tcolorbox}
[colback=white,colframe=black,left=1mm,right=1mm,top=1mm,bottom=1mm]
\ttfamily
<image>

What are the coordinates of the \{object\} in this image?

Please provide the bounding box coordinates of the \{object\} in the format: <|box\_start|>(x1, y1),(x2, y2)<|box\_end|>, where (x1, y1) for upper-left, and (x2, y2) for lower-right. All coordinates should be normalized to a [0, 1000] scale, where x corresponds to the horizontal axis (image width), y corresponds to the vertical axis (image height).
\end{tcolorbox}


\paragraph{Pixmo-Point \& Where2Place.} For these two benchmarks~\cite{deitke2024molmo,yuan2024robopoint}, we compute the proportion of predicted points that fall within the referring objects.
\begin{tcolorbox}
[colback=white,colframe=black,left=1mm,right=1mm,top=1mm,bottom=1mm]
\ttfamily
<image>

Locate several points for the \{object\}.

You can mark them using <point>x y</point>.

Please provide point coordinates in the format: <point>(x1, y1)</point> ... 

The coordinates of the point (x, y) must be **normalized to the range [0, 1000]**, where:

- x refers to the horizontal axis (image width) 
- y refers to the vertical axis (image height)

\end{tcolorbox}



\paragraph{VisualWebBench.} We use the official metric of VisualWebBench~\cite{liu2024visualwebbench}.

\begin{tcolorbox}
[colback=white,colframe=black,left=1mm,right=1mm,top=1mm,bottom=1mm]
\ttfamily
% \textbf{Appearance Order}

<image>

\texttt{\{question\}}

\end{tcolorbox}


\paragraph{ERQA.} We report accuracy on ERQA~\cite{team2025gemini}.

\begin{tcolorbox}
[colback=white,colframe=black,left=1mm,right=1mm,top=1mm,bottom=1mm]
\ttfamily
% \textbf{Appearance Order}

<image>...<image>

\texttt{\{question\}}

\{options\}

Please answer directly with only the letter of the correct option and nothing else.

\end{tcolorbox}

\paragraph{RoboVQA \& EgoTaskQA \& OpenEQA-hm3d \& OpenEQA-scannet.} We compute accuracy by using GPT-4o to compare model responses with the ground-truth labels, and the evaluation prompt is shown below. %The evaluator outputs 1 if the response matches the answer exactly or with synonymous/equivalent wording, and 0 if the response is incorrect, contradictory, or refers to a different entity, object, or attribute.

\begin{tcolorbox}
[breakable,colback=white,colframe=black,left=1mm,right=1mm,top=1mm,bottom=1mm,fontupper=\small]
\ttfamily
% \textbf{Appearance Order}

<video>

\texttt{\{question\}}

\end{tcolorbox}

\begin{tcolorbox}
[breakable,colback=white,colframe=black,left=1mm,right=1mm,top=1mm,bottom=1mm,fontupper=\small]
\ttfamily

\textbf{Prompt for GPT-4o (RoboVQA \& EgoTaskQA).}

You are an AI assistant tasked with evaluating whether a response matches the correct answer to a given question.
\vspace{1em}

\textbf{Evaluation Rules}

(1) Output 1 if the response matches the answer exactly or with synonymous/equivalent wording.

- Synonyms, paraphrases, or different surface forms of the same meaning count as matches.

- Minor wording differences (e.g., ``put tomato into fridge'' vs. ``the person is putting a tomato in the fridge'') count as matches.

\vspace{1em}

(2) Output 0 if the response is incorrect, contradictory, or refers to a different entity, object, or attribute.

- If the answer and response describe different objects, actions, or states, mark as 0.

- If the response introduces additional details that change the meaning of the answer, mark as 0.
\vspace{1em}

\textbf{Special Cases}

- Similar meaning: Output 1 if the response conveys essentially the same meaning as the answer and does not omit or add critical information (e.g., answer:``put meat on the table'', response:``The person moved meat from the fridge to the counter.'').

- Partial matches: If the response overlaps but misses or alters essential details (e.g., answer:``put meat and tomato on the table'' vs. response:``put meat on the table''), output 0.

- Granularity differences: If the response is more specific but still semantically equivalent (e.g., answer:``woman'', response:``Jessica''), output 1.

- Yes/No questions: Only output 1 if the polarity matches (yes <-> yes, no <-> no). Any mismatch outputs 0, regardless of explanation.

- Ambiguity: If the response cannot be reasonably interpreted as equivalent to the answer, output 0.

\vspace{1em}

\textbf{Examples}

Example 1

Question: Did the attribute of plant changed because of the action getting something from something?

Answer: yes

Response: Yes, the attribute of plant got watered from no to yes after the action getting something from something.

Your output: 1

\vspace{1em}

Example 2
Question: what status of fork changed while the person do the first action did before he/she put something to something?

Answer: cleanliness

Response: fork was in drawer before the person put fork to sink.

Your output: 0

\vspace{1em}

Example 3

Question: What is the person doing before he/she close something?

Answer: Put tomato to fridge

Response: The person is putting a tomato in the fridge.

Your output: 1

\vspace{1em}

Example 4

Question: What is the first action the person did in the video?

Answer: Work on sofa

Response: The person pulled out a chair.

Your output: 0

\vspace{1em}

Example 5

Question: How did the person changed the spatial relationships of meat?

Answer: Put meat to table

Response: The person moved meat from the fridge to the counter.

Your output: 1

\vspace{1em}

Example 6

Question: what status of fridge changed while the person do the first action did after he/she point to something?

Answer: openess

Response: The fridge was closed before the person point to something, and after that the fridge changed to open.

Your output: 1

\vspace{1em}

Example 7

Question: which object changed its status when the person do the last action in the video?

Answer: fork

Response: spoon

Your output: 0

\vspace{1em}

Example 8

Question: What is the action that just happened?

Answer: Place can in the tray

Response: The person puts the can on the table.

Your output: 0

\vspace{1em}

Example 9

Question: current goal is: Please place the fruits in the bowl then place the kitchen supplies into the holder. last 20 steps: 1. put white packet in the bowl 2. put white packet in the bowl 3. put yellow packet in the bowl 4. put blue packet in the bowl 5. put blue packet in the bowl 6. put blue packet in the bowl 7. put yellow packet in the bowl. What's the immediate next step?

Answer: Put duster in the black stand

Response: put brush in the holder

Your output: 0

\vspace{1em}


Your Turn:

Question: \{question\}

Answer: \{answer\}

Response: \{prediction\}

Your output:
\end{tcolorbox}

\begin{tcolorbox}
[breakable,colback=white,colframe=black,left=1mm,right=1mm,top=1mm,bottom=1mm,fontupper=\small]
\ttfamily

\textbf{Prompt for GPT-4o (OpenEQA-hm3d \& OpenEQA-scannet).}
You are an AI assistant tasked with evaluating whether a response matches the correct answer to a given question, considering both the primary answer and any extra correct answers.

\vspace{1em}

\textbf{\#\#Evaluation Rules}

(1) Output 1 if the response matches the answer or any of the extra answers exactly or with synonymous/equivalent wording.

- Synonyms, paraphrases, or different surface forms of the same meaning count as matches.

- Minor wording differences (e.g., ``Wood panel'' vs. ``Wood) count as matches.

(2) Output 0 if the response is incorrect, contradictory, or refers to a different entity, object, or attribute than the answer and all extra answers.

- If the answer and response describe different objects, actions, or states, mark as 0.

- If the response introduces additional details that change the meaning of the answer, mark as 0.

\vspace{1em}

\textbf{\#\#Special Cases}

- Similar meaning: Output 1 if the response conveys essentially the same meaning as the answer and does not omit or add critical information (e.g., answer: ``A ceiling fan'', response: ``fan'').

- Partial matches: If the response overlaps but misses or alters essential details (e.g., answer: ``put meat and tomato on the table'' vs. response: ``put meat on the table''), output 0.

- Granularity differences: If the response is more specific but still semantically equivalent (e.g., answer: ``woman'', response: ``Jessica''), output 1.

- Yes/No questions: Only output 1 if the polarity matches (yes <-> yes, no <-> no). Any mismatch outputs 0, regardless of explanation.

- Ambiguity: If the response cannot be reasonably interpreted as equivalent to the answer, output 0.

\vspace{1em}

\textbf{\#\#Examples:}

Example 1:

Question: Is it overcast?

Answer: no

Extra Answers: ["doesn't look like it", "no", "it's sunny"]

Response: yes

Your output: 0

\vspace{1em}

Example 2:

Question: Who is standing at the table?

Answer: woman

Extra Answers: ["a woman", "a lady", "woman"]

Response: Jessica

Your output: 1

\vspace{1em}

Example 3:

Question: Are there drapes to the right of the bed?

Answer: yes

Extra Answers: ["yes, there are drapes", "yeah", "the drapes are to the right of the king bed"]

Response: yes

Your output: 1

\vspace{1em}

Example 4:

Question: What material is the ceiling in the living room?

Answer: Wood panel

Extra Answers: null

Response: wood

Your output: 1

\vspace{1em}

Example 5:

Question: What is in between the two picture frames on the blue wall in the living room?

Answer: The TV

Extra Answers: null

Response: air conditioner

Your output: 0

\vspace{1em}

Example 6:

Question: Is the house doorway open or closed?

Answer: Open

Extra Answers: null

Response: The house doorway is open.

Your output: 1

\vspace{1em}

Example 7:

Question: Is my backyard safe to let me dog out in?

Answer: Yes, its fenced.

Extra Answers: null

Response: yes

Your output: 1

\vspace{1em}

Example 8:

Question: What is hanging from the ceiling in the bedroom?

Answer: A ceiling fan

Extra Answers: null

Response: fan

Your output: 1

\vspace{1em}

Example 9:

Question: Where is the full body mirror?

Answer: In the bedroom by the door

Extra Answers: ["next to the bedroom door", "just inside the bedroom", "in the bedroom", "in the bedroom right next to the door"]

Response: The full body mirror is in the bedroom.

Your output: 1

\vspace{1em}

Example 10:

Question: What is leaning in the corner by the coat rack?

Answer: An umbrella

Extra Answers: null

Response: chair

Your output: 0

\vspace{1em}

Your Turn:

Question: \{question\}

Answer: \{answer\}

Extra Answers: \{extra\_answers\}

Response: \{prediction\}

Your output: 

\end{tcolorbox}
% \paragraph{OpenEQA-hm3d.} 

% \begin{tcolorbox}
% [colback=white,colframe=black,left=1mm,right=1mm,top=1mm,bottom=1mm]
% \ttfamily
% % \textbf{Appearance Order}

% <video>

% \texttt{\{question\}}

% \end{tcolorbox}

% \paragraph{OpenEQA-scannet.} 

% \begin{tcolorbox}
% [colback=white,colframe=black,left=1mm,right=1mm,top=1mm,bottom=1mm]
% \ttfamily
% % \textbf{Appearance Order}

% <video>

% \texttt{\{question\}}

% \end{tcolorbox}


\paragraph{AgiBot-ER.} We curate 97, 120, 381 test samples for three sub-tasks, $i.e.$, Task Status Verification, Action Affordance, and Next Action Prediction, respectively.  We report the average accuracy of the three tasks.


% Specifically, we leverage a language model to generate alternative options that are slightly different from the correct one for Task Status Verification. For other two tasks, the synthetic pipeline is described in  described Section~\label{aapx:er}, where the curated benchmark is separate from the training dataset.

\begin{tcolorbox}
[colback=white,colframe=black,left=1mm,right=1mm,top=1mm,bottom=1mm]
\ttfamily
\textbf{Task Status Verification}

<image><image><image><image><image><image>

\texttt{\{question\}}

%\begin{CJK*}{UTF8}{gbsn}
\texttt{Your answer can only be "yes" or "no"}
\vspace{1em}

\textbf{Action Affordance}

<image><image><image>

\texttt{\{question\}}

\texttt{Your answer can only be "yes" or "no"}.
\vspace{1em}

\textbf{Next Task Prediction}

<image><image><image><image><image><image>

\texttt{\{question\}}

\{options\}

% Please answer directly with only the letter of the correct option and nothing else.
%\begin{CJK*}{UTF8}{gbsn}
\texttt{Answer with the option’s letter from the given choices directly.}
%\end{CJK*}


%\begin{CJK*}{UTF8}{gbsn}
%    \texttt{你的答案只能是"可以执行"或者"不可以执行"。}
%\end{CJK*}




%\end{CJK*}

% \vspace{1em}
\end{tcolorbox}


\paragraph{MME.} We report the \textit{accuracy+} metric for MME~\cite{fu2024mme}.

\begin{tcolorbox}
[colback=white,colframe=black,left=1mm,right=1mm,top=1mm,bottom=1mm]
\ttfamily
% \textbf{Appearance Order}

<image>

\texttt{\{question\}}

Please answer yes or no.

\end{tcolorbox}

\paragraph{MMBench.} We demonstrate the official metric provide by MMBench~\cite{liu2024mmbench}.

\begin{tcolorbox}
[colback=white,colframe=black,left=1mm,right=1mm,top=1mm,bottom=1mm]
\ttfamily
% \textbf{Appearance Order}

<image>

\texttt{\{question\}}

\{options\}

Answer with the option's letter from the given choices directly.

\end{tcolorbox}

\paragraph{RealWorldQA.} We use the official metric of RealWorldQA~\cite{realworldqa}.

\begin{tcolorbox}
[colback=white,colframe=black,left=1mm,right=1mm,top=1mm,bottom=1mm]
\ttfamily
% \textbf{Appearance Order}

<image>

\texttt{\{question\}}

\{options\}

Please answer directly with only the letter of the correct option and nothing else.

\end{tcolorbox}

\paragraph{SimpleVQA.} We compute accuracy by leveraging GPT-4o to compare responses against the ground-truth labels.

\begin{tcolorbox}
[colback=white,colframe=black,left=1mm,right=1mm,top=1mm,bottom=1mm]
\ttfamily
% \textbf{Appearance Order}

<image>

\texttt{\{question\}}

\end{tcolorbox}

\paragraph{EgoSchema \& VideoMME \& NextQA.} We set the number of video frames to 128 and evaluate accuracy on the three video understanding benchmarks.

\begin{tcolorbox}
[colback=white,colframe=black,left=1mm,right=1mm,top=1mm,bottom=1mm]
\ttfamily
% \textbf{Appearance Order}

<video>

\texttt{\{question\}}

\{options\}

Answer with the option's letter from the given choices directly.

\end{tcolorbox}

% \paragraph{VideoMME.} 

% \begin{tcolorbox}
% [colback=white,colframe=black,left=1mm,right=1mm,top=1mm,bottom=1mm]
% \ttfamily

% <video>

% \texttt{\{question\}}

% Answer with the option's letter from the given choices directly.

% \texttt{\{question\}}

% \end{tcolorbox}

% \paragraph{NextQA.} 

% \begin{tcolorbox}
% [colback=white,colframe=black,left=1mm,right=1mm,top=1mm,bottom=1mm]
% \ttfamily

% <video>

% \texttt{\{question\}}

% Answer with the option's letter from the given choices directly.

% \end{tcolorbox}

\paragraph{MathVista.} We use the official metric of MathVista~\cite{lu2023mathvista}.

\begin{tcolorbox}
[colback=white,colframe=black,left=1mm,right=1mm,top=1mm,bottom=1mm]
\ttfamily
% \textbf{Appearance Order}

<image>

\texttt{\{question\}}

\end{tcolorbox}

\paragraph{MathVision.} We use the official metric of MathVision~\cite{wang2024measuring}.

\begin{tcolorbox}
[colback=white,colframe=black,left=1mm,right=1mm,top=1mm,bottom=1mm]
\ttfamily

<image>

\texttt{\{question\}}

\{options\}

Please only output your final answer or a single letter (if it is a multiple choice question).

\end{tcolorbox}

\paragraph{MMMU.} We use the official metric of MMMU~\cite{yue2024mmmu}.

\begin{tcolorbox}
[colback=white,colframe=black,left=1mm,right=1mm,top=1mm,bottom=1mm]
\ttfamily

<image>

\texttt{\{question\}}

\{options\}

Answer with the option's letter from the given choices directly.

\end{tcolorbox}




\subsection{The AGIBot offline evaluation set}
\label{appx:agibot}
We select 16 high-frequency daily tasks from the AGIBot dataset for offline evaluation: ``Heat food in the microwave oven,'' ``Make a sandwich,'' ``Wash dishes with dishwasher,'' ``Wash the dishes and silverware,'' ``Discard the trash on the coffee table,'' ``Pick up the item to wipe away the stain,'' ``Place items from the meeting room table into the storage box,'' ``Arrange sofa,'' ``Wash clothes in the washing machine,'' ``Remove clothes from the washing machine,'' ``Arrange flowers,'' ``Boil water in the kettle,'' ``Packing in the supermarket,'' ``Scan and package the goods,'' ``Restock the hanging basket area,'' and ``Restock supermarket snacks.'' To ensure fairness, the data for these tasks are excluded from both the pretraining and fine-tuning datasets.


\subsection{Offline evaluation examples}
\label{appendix:offline_example}

We present a snapshot of our offline evaluation sets.

\begin{tcolorbox}
[breakable,boxrule=0pt,colback=white,left=1mm,right=1mm,top=1mm,bottom=1mm,fontupper=\small]
\ttfamily
[

    \hspace{2em}...

    \hspace{2em} \{
    
    \hspace{4em}    "role": "user",
        
    \hspace{4em}    "content": "<|system\_info\_start|>Your current views are<image><image><image><|system\_info\_end|><|human\_start|>I want some fruit, put all fruits into the basket.<|human\_end|>"
        
    \hspace{2em} \},
    
    \hspace{2em} \{
        
        \hspace{4em} "role": "assistant",
        
        \hspace{4em} "content": "<|think\_start|>...<|think\_end|><|plan\_start|>put the banana into the plastic box<|plan\_end|><|response\_start|>...<|response\_end|>",
        
        \hspace{4em}"other\_actions": [
            "put the grapes into the plastic box"
        ]
        
    \hspace{2em} \},

    \hspace{2em} \{
    
    \hspace{4em}    "role": "user",
        
    \hspace{4em}    "content": "<|system\_info\_start|>Your current views are<image><image><image><|system\_info\_end|><|human\_start|>Wait, I don't want banana.<|human\_end|>"
        
    \hspace{2em} \},

    \hspace{2em} \{
        
        \hspace{4em} "role": "assistant",
        
        \hspace{4em} "content": "<|think\_start|>...<|think\_end|><|plan\_start|>put the banana on the table<|plan\_end|><|response\_start|>...<|response\_end|>",
        
        \hspace{4em}"other\_actions": [
        ]
        
    \hspace{2em} \},
    
    \hspace{2em}...
    
]
\end{tcolorbox}

The above example illustrates two consecutive rounds  within a trajectory. We query VLMs in a manner analogous to multi-turn dialogue interactions.
For the first round, planning is considered correct if the VLM output semantically matches either: \texttt{<|plan\_start|>put the banana into the plastic box<|plan\_end|>} or \texttt{<|plan\_start|>put the grapes into the plastic box<|plan\_end|>}. 
For the second round, we evaluate models under a teacher-forcing setting, incorporating the ground-truth from the first round into the dialogue history. Since the other\_actions list is empty for this step, planning is deemed correct only if the VLM output semantically matches:
\texttt{<|plan\_start|>put the banana on the table<|plan\_end|>}.


\subsection{Online evaluation tasks}
\label{appendix:task_description}

\begin{figure}[t]
    \centering % 使图片整体居中
    
    % 第一张图片，宽度设为文本宽度的1/5，保留适当间距
    % \includegraphics[width=0.18\textwidth]{images/eval_tasks/table_clean.png}
    \begin{subfigure}{0.19\textwidth}
        \centering
        \includegraphics[width=\textwidth]{images/eval_tasks/table_clean.png}
        \caption{}
        \label{subfig:table_bussing}
    \end{subfigure}
    \begin{subfigure}{0.19\textwidth}
        \centering
        \includegraphics[width=\textwidth]{images/eval_tasks/shopping_scan_items.png}
        \caption{}
        \label{subfig:1}
    \end{subfigure}
    \begin{subfigure}{0.19\textwidth}
        \centering
        \includegraphics[width=\textwidth]{images/eval_tasks/open_end.png}
        \caption{}
        \label{subfig:1}
    \end{subfigure}
    \begin{subfigure}{0.19\textwidth}
        \centering
        \includegraphics[width=\textwidth]{images/eval_tasks/shopping_picking_items.png}
        \caption{}
        \label{subfig:1}
    \end{subfigure}
    \begin{subfigure}{0.19\textwidth}
        \centering
        \includegraphics[width=\textwidth]{images/eval_tasks/table_clean_and_ship_items.png}
        \caption{}
        \label{subfig:shipment}
    \end{subfigure}
    \caption{Example initial states of the five tasks used in our online evaluation. (a) Table bussing: removing used dishes, utensils, and food items; (b) Checkout packing: organizing and placing purchased items into bags or boxes at checkout; (c) Dietary filtering: selecting or excluding food and drink items based on dietary constraints; (d) Grocery shopping: retrieving and collecting grocery items according to user instructions; (e) Tableware organization \& shipment: sorting, packing, and transporting tableware to designated locations.}
    \label{fig:online_eval_tasks} % 用于交叉引用的标签
\end{figure}

Example initial states of the five tasks used in our online evaluation are shown in \Cref{fig:online_eval_tasks}. Below, we provide an overview of each task.
\begin{itemize}[leftmargin=0.5cm]
    \item \textbf{Table bussing}: removing used dishes, utensils, and food items. In our experiment, the user requests the robot to clear the table, but interrupts with the command ``\textit{I still need it}'' while the robot is placing a glass into the plastic box. We also introduce a failure event when the robot attempts to place a spoon into the box.
    \item \textbf{Checkout packing}: organizing and placing purchased items into bags or boxes at checkout. In our experiment, the user asks the robot to move all items on the checkout counter into the shopping basket. An interruption occurs with the command ``\textit{I am allergic to caffeine}'' while the robot is placing a coffee into the basket.
    \item \textbf{Dietary filtering}: selecting or excluding food and drink items based on dietary constraints (e.g., no caffeine, vegetarian). In our experiment, the user issues a series of instructions: (1) ``\textit{Put the food with the highest energy into the plastic box, then add a drink. Note that I am allergic to caffeine.}''; (2) ``\textit{Discard all drinks containing caffeine into the rubbish bin}''; (3) ``\textit{Place all fruits and vegetables into the plastic box}''; and (4) ``\textit{Clean up all remaining items on the table}''.
    \item \textbf{Grocery shopping}: retrieving and collecting grocery items according to user instructions. In our experiment, the user first asks the robot to recommend a snack suitable for a road trip. Following the recommendation, the user requests a less sweet snack for the cart, then asks for a non-alcoholic drink, and finally makes a conditional request: ``Are there any nuts on the shelf? If so, put some into the shopping cart.''
    \item \textbf{Tableware organization \& shipment} : sorting, packing, and transporting tableware to designated locations. In our experiment, the user instructs the robot to discard all trash and transport the tableware to the sink. Specifically, the robot must first dispose of garbage in the rubbish bin, then place all tableware into a plastic box, and finally carry the box to the sink. During this process, the user interrupts with the command ``\textit{Keep it on the table}'' while the robot is placing a stainless steel cup into the box.
\end{itemize}

\subsection{Offline \& Online Evaluation Prompts}

\label{appendix:prompts}

We present the prompts used in our experiments, including the judge prompt for offline evaluation, the baseline model prompts, and the reward model prompt for reinforcement learning.

\textbf{Judge Prompt for Offline Evaluation}
\begin{tcolorbox}
[breakable,colback=white,colframe=black,left=1mm,right=1mm,top=1mm,bottom=1mm,fontupper=\small]
\ttfamily

\# Role

You are a judge to decide the similarity of two sentences.

\vspace{1em}

\# Inputs

You will be provided with two sentences, each sentence represent an action from a robot.

\vspace{1em}

\# Output Format

Your output should be a single number that is either 0 or 1, where 0 means the two sentences are semantically different, and 1 means the two sentences are semantically the same. Output in the following format: "[SOME ANALYSIS]. The final answer is: [NUMBER]"

\vspace{1em}

\# Examples

User:

1. put the fork into the basket

2. put the fork into the basket

Assistant:

Two sentences are exactly the same. The final answer is: 1.0

\vspace{1em}

User:

1. put the iron fork into the woven basket

2. put the fork into the basket

Assistant:

Two sentences are the same semantically. The final answer is: 1.0

\vspace{1em}

User:

1. Grab the bottled french fries on the table with the right arm.

2. Grab the bottled french fries.

Assistant:

Two sentences are the same semantically. The final answer is: 1.0

\vspace{1em}

User:

1. Move forward slightly

2. Move forward

Assistant:

Two sentences are the same semantically. The final answer is: 1.0

\vspace{1em}

User:

1. put the coffee into the plastic box

2. put the bottle of coffee into the plastic box

Assistant:

Two sentences are the same semantically. The final answer is: 1.0

\vspace{1em}

User:

1. put the glass into the plastic box

2. put the glass cup into the plastic box

Assistant:

Two sentences are the same semantically. The final answer is: 1.0

\vspace{1em}

User:

1. put the fork into the basket

2. put the knife into the basket

Assistant:

The objects (fork v.s. knife) are different semantically. The final answer is: 0.0

\vspace{1em}

User:

1. put the fork into the basket

2. pick up the fork

Assistant:

The actions are different semantically. The final answer is: 0.0

\vspace{1em}

User:

1. put the fork into the basket

2. navigate to the table

Assistant:

Neither actions nor objects matches. The final answer is: 0.0

\vspace{1em}

User:

1. put the fork into the basket

2. pick up the stainless steel cup

Assistant:

Neither actions nor objects matches. The final answer is: 0.0

\end{tcolorbox}

% \begin{tcolorbox}[
%     title=Judge prompt,
%     breakable,          % 关键：启用自动分页
%     colback=white,      % 背景色
%     colframe=blue!50,   % 边框色
%     fonttitle=\bfseries,
%     before skip=10pt,   % 上方间距
%     after skip=10pt,     % 下方间距
%     fontupper=\scriptsize
% ]
% \begin{lstlisting}
% # Role
% You are a judge to decide the similarity of two sentences.

% # Inputs
% You will be provided with two sentences, each sentence represent an action from a robot.

% # Output Format
% Your output should be a single number that is either 0 or 1, where 0 means the two sentences are semantically different, and 1 means the two sentences are semantically the same. Output in the following format: "[SOME ANALYSIS]. The final answer is: [NUMBER]"

% # Examples
% User:
% 1. put the fork into the basket
% 2. put the fork into the basket
% Assistant:
% Two sentences are exactly the same. The final answer is: 1.0

% User:
% 1. put the iron fork into the woven basket
% 2. put the fork into the basket
% Assistant:
% Two sentences are the same semantically. The final answer is: 1.0

% User:
% 1. Grab the bottled french fries on the table with the right arm.
% 2. Grab the bottled french fries.
% Assistant:
% Two sentences are the same semantically. The final answer is: 1.0

% User:
% 1. Move forward slightly
% 2. Move forward
% Assistant:
% Two sentences are the same semantically. The final answer is: 1.0

% User:
% 1. put the coffee into the plastic box
% 2. put the bottle of coffee into the plastic box
% Assistant:
% Two sentences are the same semantically. The final answer is: 1.0

% User:
% 1. put the glass into the plastic box
% 2. put the glass cup into the plastic box
% Assistant:
% Two sentences are the same semantically. The final answer is: 1.0

% User:
% 1. put the fork into the basket
% 2. put the knife into the basket
% Assistant:
% The objects (fork v.s. knife) are different semantically. The final answer is: 0.0

% User:
% 1. put the fork into the basket
% 2. pick up the fork
% Assistant:
% The actions are different semantically. The final answer is: 0.0

% User:
% 1. put the fork into the basket
% 2. navigate to the table
% Assistant:
% Neither actions nor objects matches. The final answer is: 0.0

% User:
% 1. put the fork into the basket
% 2. pick up the stainless steel cup
% Assistant:
% Neither actions nor objects matches. The final answer is: 0.0
% \end{lstlisting}
% \end{tcolorbox}


\textbf{English Prompt for Baseline Models.}

We use the following prompt to configure VLMs as the interaction and planning modules of the robot system in both offline and online experiments.
\begin{tcolorbox}
[breakable,colback=white,colframe=black,left=1mm,right=1mm,top=1mm,bottom=1mm,fontupper=\small]
\ttfamily
\# Role

You are a robot with two grippers developed by Bytedance, and your name is Roobio. You are deployed in a home environment, and your job is to have natural interactions with users and complete some tasks required by the user.

You have basic movement, perception, and manipulation capabilities, and can navigate to the following areas: dining table, sink, refrigerator, dishwasher, microwave, bread maker, cupboard, shoe cabinet, sofa, and washing machine.

\vspace{1em}

\# Input

In each round, you will be provided with the following information.

1. Three images: captured by the cameras from your head/left gripper/right gripper respectively. These images reflect your current visual perception at the current moment.

2. User instructions (optional): user may give you some instructions, user instructions are in chinese.

\# Output

To distinguish reasoning, planning, response and query. You must output with the following fields.

1. `<|think\_start|> ... <|think\_end|>': this field is for your reasoning process, it can include

\hspace{2em}    - The key items in the current scene.

\hspace{2em}    - Whether the previous action is complete.
    
\hspace{2em}    - Reasoning about your next action.

2. `<|plan\_start|> ... <|plan\_end|>' (optional): this field is for task planning, You should plan your next action based on your reasoning process. The action should be helpful to complete user's task.

3. `<|response\_start|> ... <|response\_end|>' (optional): this field is your response to user, you response must be in *chinese*. You should respond to the user in the following situations.
    
\hspace{2em}    - When the user is chatting with you;
    
\hspace{2em}    - When the user gives a new instruction on completing a task, you should always respond to the user whenever you receive a new instruction. The response should be concise, polite, and relevant to the task.
    
\hspace{2em}    - When you need to ask the user for more information. For example, if the user ask you to give him/her a drink, and you observe both orange juice and apple juice, then you should ask the user which one he/she prefers. You should avoid asking the user for more information too frequently.

\vspace{1em}

\# Guidelines

1. The text inside `<|think\_start|> ... <|think\_end|>' and `<|plan\_start|> ... <|plan\_end|>' should be in english while the text in `<|response\_start|> ... <|response\_end|>' must be in chinese.

2. When the user interrupt your action, you need to stop the current action and re-plan.

3. Your task planning inside `<|plan\_start|> ... <|plan\_end|>' should be in the following format:

\hspace{2em}    - put the ... into the ...

\hspace{2em}    - pick up the ...

\hspace{2em}    - navigate to the ...

\hspace{2em}    - open the ...

\hspace{2em}    - close the ...

4. Only include one action at a time, planning such as `<|plan\_start|> put the A into the B, put the C into the B<|plan\_end|>' is invalid.

\vspace{1em}

\# Examples

User:

<|system\_info\_start|>Your current views are...<|system\_info\_end|><|human\_start|>Robot, clean up the table for me.<|human\_end|>

Assistant:

<|think\_start|>The user asks me to clean up the table, I can observe.... <|think\_end|><|plan\_start|>put the ... into the ...<|plan\_end|><|response\_start|>...<|response\_end|>

User:

<|system\_info\_start|>The views you see after finishing previous action are...<|system\_info\_end|>

Assistant:

<|think\_start|>I should continue cleaning up the table, there are ... left on the table, ...<|think\_end|><|plan\_start|>put the ... into the ...<|plan\_end|>

...
\end{tcolorbox}

\textbf{Chinese Prompt for Baseline Models}

We also developed a corresponding Chinese prompt for models that perform better with Chinese.
\begin{tcolorbox}
[breakable,colback=white,colframe=black,left=1mm,right=1mm,top=1mm,bottom=1mm,fontupper=\small]
\ttfamily
\begin{CJK*}{UTF8}{gbsn}
    \texttt{\# 角色}
\end{CJK*}

\begin{CJK*}{UTF8}{gbsn}
    \texttt{你是字节跳动研发的双臂机器人。你被部署在一个开放式厨房环境中，负责与人类用户进行自然互动并完成日常操作任务。你具备基础的移动、感知与操控能力，可前往以下区域执行操作：餐桌旁、水池旁、冰箱旁、洗碗机旁、微波炉旁、烤面包机旁、水池旁的台面、鞋柜旁、沙发旁和洗衣机旁。}
\end{CJK*}

\vspace{1em}

\begin{CJK*}{UTF8}{gbsn}
    \texttt{\# 输入信息}
\end{CJK*}

\begin{CJK*}{UTF8}{gbsn}
    \texttt{在每轮交互中，你将接收到以下信息：}
\end{CJK*}

\begin{CJK*}{UTF8}{gbsn}
    \texttt{（1）三张图像：分别来自你头部摄像头、左夹爪摄像头、右夹爪摄像头，反映你在当前时刻的视觉感知。}
\end{CJK*}

\begin{CJK*}{UTF8}{gbsn}
    \texttt{（2）用户指令（可选）：人类用户可能通过语音或文本向你发出任务指令。}
\end{CJK*}

\vspace{1em}


\begin{CJK*}{UTF8}{gbsn}
    \texttt{\# 输出格式}
\end{CJK*}

\begin{CJK*}{UTF8}{gbsn}
    \texttt{你必须输出以下结构化内容，用于指导任务执行与用户交互。输出字段包括：}
\end{CJK*}

\begin{CJK*}{UTF8}{gbsn}
    \texttt{（1）<|think\_start|> ... <|think\_end|>：你的内部思考与任务状态判断，包括：}
\end{CJK*}

\begin{CJK*}{UTF8}{gbsn}
    \texttt{\hspace{2em}- 当前场景中包含的关键物品；}
\end{CJK*}

\begin{CJK*}{UTF8}{gbsn}
    \texttt{\hspace{2em}- 是否完成上一步操作；}
\end{CJK*}

\begin{CJK*}{UTF8}{gbsn}
    \texttt{\hspace{2em}- 当前场景变化的观察；}
\end{CJK*}

\begin{CJK*}{UTF8}{gbsn}
    \texttt{\hspace{2em}- 下一步应执行的关键动作与理由；}
\end{CJK*}

\begin{CJK*}{UTF8}{gbsn}
    \texttt{\hspace{2em}- 如遇异常（如抓取失败），应在此说明并调整策略。}
\end{CJK*}

\begin{CJK*}{UTF8}{gbsn}
    \texttt{（2）<|plan\_start|> ... <|plan\_end|>（可选）：你对下一步具体动作的操作规划，目标是完成当前用户任务。操作步骤应使用英文简洁描述。}
\end{CJK*}

\begin{CJK*}{UTF8}{gbsn}
    \texttt{（3）<|response\_start|> ... <|response\_end|>（可选）：你对用户的语音或文本形式的自然语言回复，内容需简洁、礼貌并与任务状态相关。当当前信息不足以明确执行用户任务时，你可以主动向用户提问以获取更多信息。但请遵循``非必要不提问''的原则，避免频繁打断用户。}
\end{CJK*}

\vspace{1em}


\begin{CJK*}{UTF8}{gbsn}
    \texttt{\# 任务规则}
\end{CJK*}

\begin{CJK*}{UTF8}{gbsn}
    \texttt{在于用户的交互与执行任务的过程中，你需要遵循以下规则：}
\end{CJK*}

\begin{CJK*}{UTF8}{gbsn}
    \texttt{（1）`<|think\_start|> ... <|think\_end|>'和`<|response\_start|> ... <|response\_end|>'中的文本以中文输出，`<|plan\_start|> ... <|plan\_end|>'中的任务规划以英文输出；}
\end{CJK*}

\begin{CJK*}{UTF8}{gbsn}
    \texttt{（2）用户可能会打断你的操作，你需要基于当前画面和用户给你的最新指令决定下一步的操作；}
\end{CJK*}

\begin{CJK*}{UTF8}{gbsn}
    \texttt{（3）`<|plan\_start|>...<|plan\_end|>'中的操作推荐遵循以下格式：}
\end{CJK*}

\hspace{2em}    - put the ... into the ...

\hspace{2em}    - pick up the ...

\hspace{2em}    - navigate to the ...

\hspace{2em}    - open the ...

\hspace{2em}    - close the ...

\begin{CJK*}{UTF8}{gbsn}
    \texttt{（4）`<|plan\_start|>...<|plan\_end|>'中的任务规划一次只能规划下一步的内容，不能规划之后多步的内容，例如：put the A to the B, put the C to the D...这样多个操作不能放到一次规划中，但是它可以出现在你的思考过程中。}
\end{CJK*}


\vspace{1em}

\begin{CJK*}{UTF8}{gbsn}
    \texttt{\# 例子}
\end{CJK*}

User:

\begin{CJK*}{UTF8}{gbsn}
    \texttt{<|system\_info\_start|>你当前看到的画面为...<|system\_info\_end|><|human\_start|>帮我清理桌面。<|human\_end|>}
\end{CJK*}

Assistant:

\begin{CJK*}{UTF8}{gbsn}
    \texttt{<|think\_start|>用户让我清理桌面，当前画面中我能看到.... <|think\_end|><|plan\_start|>put the ... into the ...<|plan\_end|><|response\_start|>收到。<|response\_end|>}
\end{CJK*}


User:

\begin{CJK*}{UTF8}{gbsn}
    \texttt{<|system\_info\_start|>你完成操作后所看到的场景为...<|system\_info\_end|>}
\end{CJK*}

Assistant:

\begin{CJK*}{UTF8}{gbsn}
    \texttt{<|think\_start|>我应该继续收拾桌面，当前我能看到桌面上还有...<|think\_end|><|plan\_start|>put the ... into the ...<|plan\_end|>
}
\end{CJK*}

...
\end{tcolorbox}


\textbf{Reward Model Prompt for RL}
\begin{tcolorbox}
[breakable,colback=white,colframe=black,left=1mm,right=1mm,top=1mm,bottom=1mm,fontupper=\small]
\ttfamily
\# Role

You are a consistency checker for a robot's planning. Your task is to evaluate the robot's thinking process and the resulting final action.

\vspace{1em}

\# Input

1. The robot's thinking process, enclosed by <|think\_start|> and <|think\_end|>.

2. The robot's final action, enclosed by <|plan\_start|> and <|plan\_end|>.

\vspace{1em}

\# Task

You need to determine:

1. Whether the thinking process within <|think\_start|> and <|think\_end|> is reasonable.

2. Whether the final decision within <|plan\_start|> and <|plan\_end|> is consistent with the decision derived from the thinking process in <|think\_start|> and <|think\_end|>.

\vspace{1em}

\# Output

Your output must follow this format: [Your reasoning process] + "The final answer is: [NUMBER]."
\vspace{0.5em}

Here, [NUMBER] is an integer: `1' indicates consistency; `-1' indicates inconsistency; `0' indicates that it is impossible to judge.

\vspace{1em}

\# Notes

1. Ignore ambiguity in names. Items that could potentially be consistent should be considered consistent.

2. Assign -1 only if the thinking process is completely unreasonable.

3. Assign -1 only if it's completely impossible for the thinking process and the plan to be consistent.

4. If the plan is only a part of the strategy outlined in the thinking process, it is still considered consistent (i.e., the plan does not need to reflect all thoughts).
\end{tcolorbox}


% \begin{tcolorbox}[
%     title=Chinese prompt,
%     breakable,          % 关键：启用自动分页
%     colback=white,      % 背景色
%     colframe=blue!50,   % 边框色
%     fonttitle=\bfseries,
%     before skip=10pt,   % 上方间距
%     after skip=10pt,     % 下方间距
%     fontupper=\scriptsize
% ]

% \begin{CJK*}{UTF8}{gbsn}
% \# \texttt{角色定义} \\
% 你是字节跳动研发的双臂机器人，名字叫 Roobio。你被部署在一个开放式厨房环境中，负责与人类用户进行自然互动并完成日常操作任务。\\
% 你具备基础的移动、感知与操控能力，可前往以下区域执行操作：餐桌旁、水池旁、冰箱旁、洗碗机旁、微波炉旁、烤面包机旁、水池旁的台面、鞋柜旁、沙发旁和洗衣机旁。 \\

% \# 输入信息
% 在每轮交互中，你将接收到以下信息：\\
% （1）三张图像：分别来自你头部摄像头、左夹爪摄像头、右夹爪摄像头，反映你在当前时刻的视觉感知。\\
% （2）用户指令（可选）：人类用户可能通过语音或文本向你发出任务指令。

% \# 输出格式
% 你必须输出以下结构化内容，用于指导任务执行与用户交互。输出字段包括：\\
% （1）\texttt{<|think\_start|> ... <|think\_end|>}：你的内部思考与任务状态判断，可以包括：
% - 当前场景中包含的关键物品；\\
% - 是否完成上一步操作；\\
% - 当前场景变化的观察；\\
% - 下一步应执行的关键动作与理由；\\
% - 如遇异常（如抓取失败），应在此说明并调整策略。\\
% （2）\texttt{<|plan\_start|> ... <|plan\_end|>}（可选）：你对下一步具体动作的操作规划，目标是完成当前用户任务。操作步骤应使用英文简洁描述。\\
% （3）\texttt{<|response\_start|> ... <|response\_end|>}（可选）：你对用户的语音或文本形式的自然语言回复，内容需简洁、礼貌并与任务状态相关。\\
% （4）\texttt{<|query\_start|> ... <|query\_end|>}（可选）：当当前信息不足以明确执行用户任务时，你可以主动向用户提问以获取更多信息。但请遵循``非必要不提问''的原则，避免频繁打断用户。\\
% （5）\texttt{<|task\_finished|>}（可选）：当任务完成后，用户明确表示没有新的需求后，直接输出\texttt{<|task\_finished|>}。\\

% \# 任务规则：在任务执行过程中，你需要遵循以下规则：\\
% （1）你可以执行的操作包括：\\
%     - put ... into ...\\
%     - pick up ...\\
%     - navigate to ...\\
%     - close ...\\
%     - open ...\\
% （2）\texttt{`<|plan\_start|>...<|plan\_end|>`}中的任务规划一次只能规划下一步的内容，不能规划之后多步的内容，例如：put the A to the B, put the C to the D...这样多个操作不能放到一次规划中，但是它可以出现在你的思考过程中（\texttt{`<|think\_start|>...<|think\_end|>`}中的内容）。\\
% （3）当你需要把A物品放到B物品中时，直接使用put the A into the B，不需要先pick up A再put the A into the B；\\

% \# 例子
% User:\\
% \texttt{<|system\_info\_start|>}你现在所看到的场景为...\texttt{<|system\_info\_end|><|human\_start|>}Roobio，收拾一下桌子。\texttt{<|human\_end|>} \\
% Assistant:\\
% \texttt{<|think\_start|>}用户让我清理桌面。我能看到桌面上有一些垃圾（...），还有一些餐具（...）。另外我还能看到...。我应该执行以下操作：- 先把垃圾扔到垃圾桶；- 把餐具收到收纳盒；- .... \texttt{<|think\_end|><|plan\_start|>}put the ... into the ...\texttt{<|plan\_end|><|response\_start|>}好的，没问题。\texttt{<|response\_end|>} \\
% User:\\
% \texttt{<|system\_info\_start|>}你完成操作后所看到的场景为...\texttt{<|system\_info\_end|>}\\
% Assistant:\\
% \texttt{<|think\_start|>}我应该继续收拾桌面，把...放进...。\texttt{<|think\_end|><|plan\_start|>}put the ... into the ...\texttt{<|plan\_end|>}\\
% ...
% \end{CJK*}

% \end{tcolorbox}

%\section{Data Synthesis Pipeline}

\section{Embodied Task-centric Reasoning}
\label{aapx:er}

\subsection{Data Synthesis}

\label{aapx:er_sub}

Publicly available robot datasets often contain long video demonstrations with temporally annotated clips and corresponding individual actions, or they can be segmented automatically into clips using VLMs. To equip \name{} with reasoning and planning capabilities in embodied scenarios, we design three dedicated synthesis pipelines, each targeting a distinct sub-task: task status verification, action affordance, and next action prediction. The details of these pipelines are provided below.

\paragraph{Task Status Verification.} The status of a task is categorized as either complete or incomplete. To construct task verification data labeled as complete, we use the entire video clip as the visual input. Reasoning traces are obtained by prompting a strong VLM (Seed-1.5-VL in thinking mode) with the question ``Is the \{action\} complete?''. We then extract the reasoning content from the response and retain only those instances where the predicted status is complete. Conversely, to represent incomplete task status, we randomly truncate each video clip to between one-half and one-third of its original duration, producing partial visual inputs. As before, we retain only those cases where the predicted status is identified as incomplete.

\paragraph{Action Affordance.} To obtain high-quality labels for action affordance, we distill both labels and reasoning traces from powerful VLMs. However, we find that relying on a single VLM is insufficient for generating accurate labels reliably. Therefore, we employ various VLMs to produce candidate labels and take the intersection of their outputs as the final annotation. The corresponding reasoning traces are extracted from the Seed-1.5-VL-Think model.

\paragraph{Next Action Prediction.} 
The robot datasets are typically annotated with action sequences. Thus, the ground-truth next action can be directly determined once the previous action is specified. To synthesize the corresponding reasoning trace, we leverage Seed-1.5-VL by prompting it with both the video and the following textual input: \textit{``You are an intelligent robot executing \{the task\}. To complete this task, you are performing the action as shown in the video. Your next action is \{next action\}. Please reflect on the rationale behind your next action and output your response from the perspective of a robotic agent.''}

\subsection{Agibot-ER Benchmark}

We construct an embodied task-centric reasoning benchmark based on the Agibot dataset~\cite{bu2025agibot}, which provides manual annotations of tasks, atomic action sequences, and the corresponding video clips for each action. Specifically:
\begin{itemize}
    \item Task Status Verification: We randomly select 100 samples from the synthesized dataset and further verify the label accuracy, resulting in 97 test samples.
    \item Action Affordance: We select 120 video clips and corresponding individual actions from 50 different tasks. To ensure accuracy, we manually annotate these samples rather than relying on VLM-based annotation.
    \item Next Action Prediction. The ground-truth next action is obtained directly from the robot datasets. We randomly sample 400 instances and construct distractor options by leveraging a powerful LLM to generate incorrect candidates that differ subtly from the correct one—such as variations in action type, target object, or destination. To ensure quality, we manually verify all synthesized options, resulting in 381 validated test samples.
\end{itemize}
All test samples are eliminated from the training dataset.





% For sub-task \textbf{Next Action Prediction}, we leverage a language model to generate alternative options that are slightly different from the correct one. For other two tasks, the synthetic pipeline is described in  described Section~\label{aapx:er}, where the curated benchmark is separate from the training dataset.


% \begin{tcolorbox}[
%     title=Chinese prompt,
%     breakable,          % 关键：启用自动分页
%     colback=white,      % 背景色
%     colframe=blue!50,   % 边框色
%     fonttitle=\bfseries,
%     before skip=10pt,   % 上方间距
%     after skip=10pt,     % 下方间距
%     fontupper=\scriptsize
% ]
% \begin{lstlisting}
% #角色定义
% 你是字节跳动研发的双臂机器人，名字叫 Roobio。你被部署在一个开放式厨房环境中，负责与人类用户进行自然互动并完成日常操作任务。
% 你具备基础的移动、感知与操控能力，可前往以下区域执行操作：餐桌旁、水池旁、冰箱旁、洗碗机旁、微波炉旁、烤面包机旁、水池旁的台面、鞋柜旁、沙发旁和洗衣机旁。

% #输入信息
% 在每轮交互中，你将接收到以下信息：
% （1）三张图像：分别来自你头部摄像头、左夹爪摄像头、右夹爪摄像头，反映你在当前时刻的视觉感知。
% （2）用户指令（可选）：人类用户可能通过语音或文本向你发出任务指令。

% #输出格式
% 你必须输出以下结构化内容，用于指导任务执行与用户交互。输出字段包括：
% （1）<|think_start|> ... <|think_end|>：你的内部思考与任务状态判断，可以包括：
% - 当前场景中包含的关键物品；
% - 是否完成上一步操作；
% - 当前场景变化的观察；
% - 下一步应执行的关键动作与理由；
% - 如遇异常（如抓取失败），应在此说明并调整策略。
% （2）<|plan_start|> ... <|plan_end|>（可选）：你对下一步具体动作的操作规划，目标是完成当前用户任务。操作步骤应使用英文简洁描述。
% （3）<|response_start|> ... <|response_end|>（可选）：你对用户的语音或文本形式的自然语言回复，内容需简洁、礼貌并与任务状态相关。
% （4）<|query_start|> ... <|query_end|>（可选）：当当前信息不足以明确执行用户任务时，你可以主动向用户提问以获取更多信息。但请遵循``非必要不提问''的原则，避免频繁打断用户。
% （5）<|task_finished|>（可选）：当任务完成后，用户明确表示没有新的需求后，直接输出<|task_finished|>

% # 任务规则：在任务执行过程中，你需要遵循以下规则：
% （1）你可以执行的操作包括：
%     - put ... into ...
%     - pick up ...
%     - navigate to ...
%     - close ...
%     - open ...
% （2）`<|plan_start|>...<|plan_end|>`中的任务规划一次只能规划下一步的内容，不能规划之后多步的内容，例如：put the A to the B, put the C to the D...这样多个操作不能放到一次规划中，但是它可以出现在你的思考过程中（`<|think_start|>...<|think_end|>`中的内容）。
% （3）当你需要把A物品放到B物品中时，直接使用put the A into the B，不需要先pick up A再put the A into the B；


% #例子
% User:
% <|system_info_start|>你现在所看到的场景为...<|system_info_end|><|human_start|>Roobio，收拾一下桌子。<|human_end|>
% Assistant:
% <|think_start|>用户让我清理桌面。我能看到桌面上有一些垃圾（...），还有一些餐具（...）。另外我还能看到...。我应该执行以下操作：\n- 先把垃圾扔到垃圾桶；\n- 把餐具收到收纳盒；\n- .... <|think_end|><|plan_start|>put the ... into the ...<|plan_end|><|response_start|>好的，没问题。<|response_end|>
% User:
% <|system_info_start|>你完成操作后所看到的场景为...<|system_info_end|>
% Assistant:
% <|think_start|>我应该继续收拾桌面，把...放进...。<|think_end|><|plan_start|>put the ... into the ...<|plan_end|>
% ...
% \end{lstlisting}
% \end{tcolorbox}


\section{Case studies of RL}\label{appx:case-study}

Our reinforcement learning stage yields several improvements over the SFT model, including: (1) reduced irrational reasoning, (2) improved thought-action consistency, and (3) fewer formatting errors. In the following, we present comparative case studies between \name{}-32B-RL and \name{}-32B-SFT to illustrate the effectiveness of reinforcement learning.


\textbf{Reduced irrational reasoning}
\begin{tcolorbox}
[breakable,colback=white,colframe=black,left=1mm,right=1mm,top=1mm,bottom=1mm,fontupper=\small]
\ttfamily
\# Current task

Put all the drinks on the table into the carton.

\vspace{1em}
\# \name{}-32B-RL output

<|think\_start|>Based on the current scene, I see that there is already a bottle of soda inside the carton, and the remaining items on the table are milk, Oreos, and gum. Recalling my last action, I have already put the coke into the carton. Now, the only beverage left on the table is milk. To complete the task of putting all beverages into the carton, the next step should be to put the milk into the carton. <|think\_end|>

<|plan\_start|>put the milk into the carton<|plan\_end|>

\vspace{1em}
\# \name{}-32B-SFT output

<|think\_start|>Based on the current scene, I see that there is already a bottle of soda inside the carton, and the remaining items on the table are milk, Oreos, and gum. Recalling my last action, I have already put the coke into the carton. Now, all the beverages on the table have been put into the carton, and the task goal has been achieved. Next, I should proactively ask the user if there are any other tasks that need assistance. <|think\_end|>

<|response\_start|>The task has been processed. Is there anything else I can help you with? <|response\_end|>
\end{tcolorbox}





\textbf{Improved thought-action consistency}
\begin{tcolorbox}
[breakable,colback=white,colframe=black,left=1mm,right=1mm,top=1mm,bottom=1mm,fontupper=\small]
\ttfamily
\# Current Task

Put the dishes in the sink

\vspace{1em}
\# \name{}-32B-RL output

<|think\_start|>I have grasped the storage basket with my dual grippers. The basket contains bowls, forks, and spoons. According to the user's instructions, the next step is to take these dishes to the sink. I have now finished collecting the tableware. Next, I should navigate to the sink area and deliver the dishes to the designated location.<|think\_end|>

<|plan\_start|>navigate to the sink<|plan\_end|>

\vspace{1em}
\# \name{}-32B-SFT output

<|think\_start|>I have grasped the storage basket with my dual grippers, ready to transport the dishes. According to the user's instructions, the dishes need to be taken to the sink. All the dishes that need to be washed have been collected in the storage basket. The next step is to transport the storage basket to the sink area, completing the task of collecting and transporting the dishes.<|think\_end|>

<|plan\_start|>navigate to the cupboard<|plan\_end|>

\end{tcolorbox}


\textbf{Fewer formatting errors}

\begin{tcolorbox}
[breakable,colback=white,colframe=black,left=1mm,right=1mm,top=1mm,bottom=1mm,fontupper=\small]
\ttfamily
\# Current Task

Organize the table

\vspace{1em}
\# \name{}-32B-RL output

<|think\_start|>From the current scene, the paper cup is still on the table, near the rubbish bin, and is grasped by my gripper, which indicates that the previous attempt to put the paper cup into the rubbish bin was not successful. Besides the paper cup, there is also a plate with some leftover food residue on the table. To continue organizing the table, I first need to re-attempt putting the paper cup into the rubbish bin to ensure the trash is handled correctly.<|think\_end|>
<|plan\_start|>put the paper cup into the rubbish bin<|plan\_end|>

\vspace{1em}
\# \name{}-32B-SFT output

<|think\_start|>From the current scene, the paper cup is still on the table, near the rubbish bin, and is grasped by my gripper, which indicates that the previous attempt to put the paper cup into the rubbish bin was not successful. Besides the paper cup, there is also a plate with some leftover food residue on the table. To continue organizing the table, I first need to re-attempt putting the paper cup into the rubbish bin to ensure the trash is handled correctly.<|think\_end|>

\begin{verbatim}
{
  "action": "put",
  "object": "paper cup",
  "target": "rubbish bin"
}
\end{verbatim}

\end{tcolorbox}
